# Supplementary material for: Geometric Epitope and Paratope Prediction
Source: arXiv:2307.13608 source file (2023-05-28)
Supplement: Supplementary file 1 [file add_results.tex]

\section{\label{sec:add_res} Additional results}

\begin{figure}[t!]
\vspace{0.2cm}
\centering
\begin{overpic}
[trim=0cm 0cm -2cm 0cm,clip,width=0.99\linewidth, grid=false]{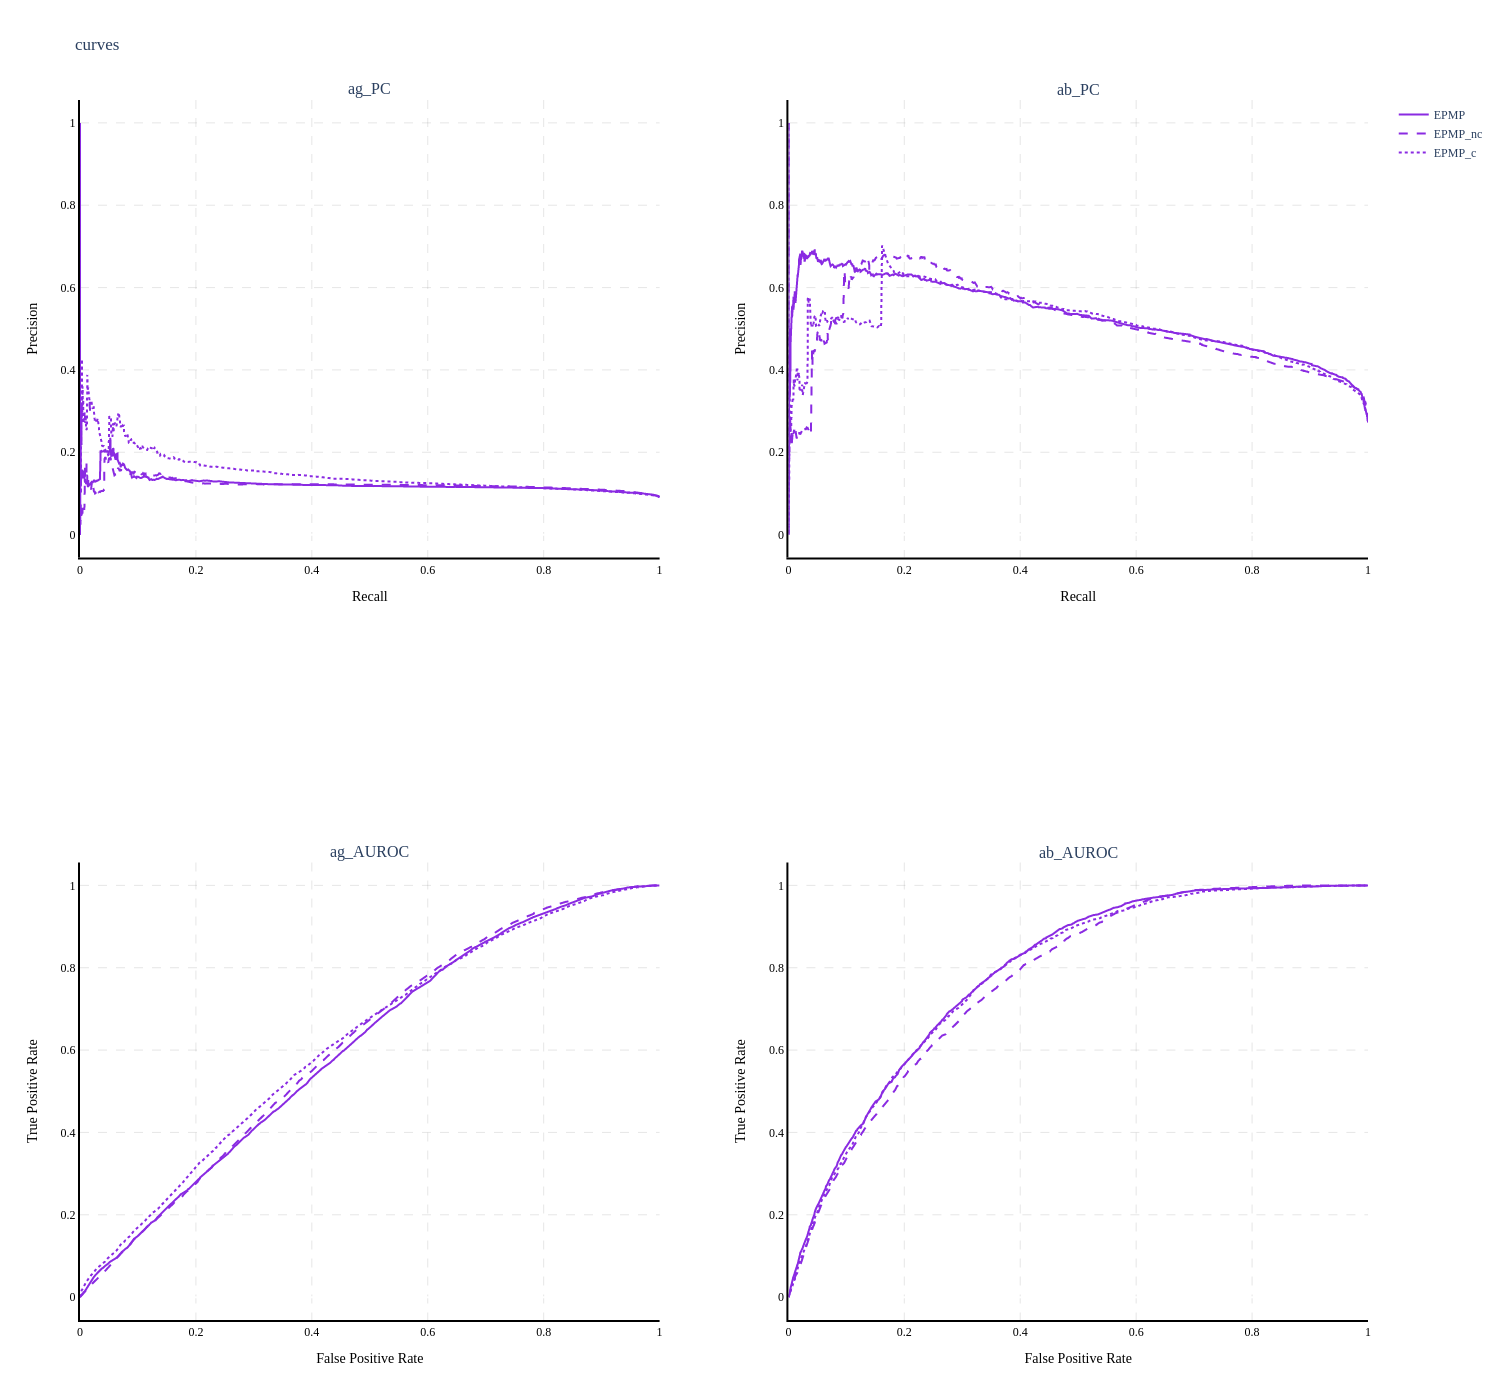}
\end{overpic}
\caption{\label{fig:graph_curves}}
\end{figure}

\begin{figure*}[t!]
\vspace{0.2cm}
\centering
\begin{overpic}
[trim=0cm 0cm -3cm 0cm,clip,width=0.99\linewidth, grid=false]{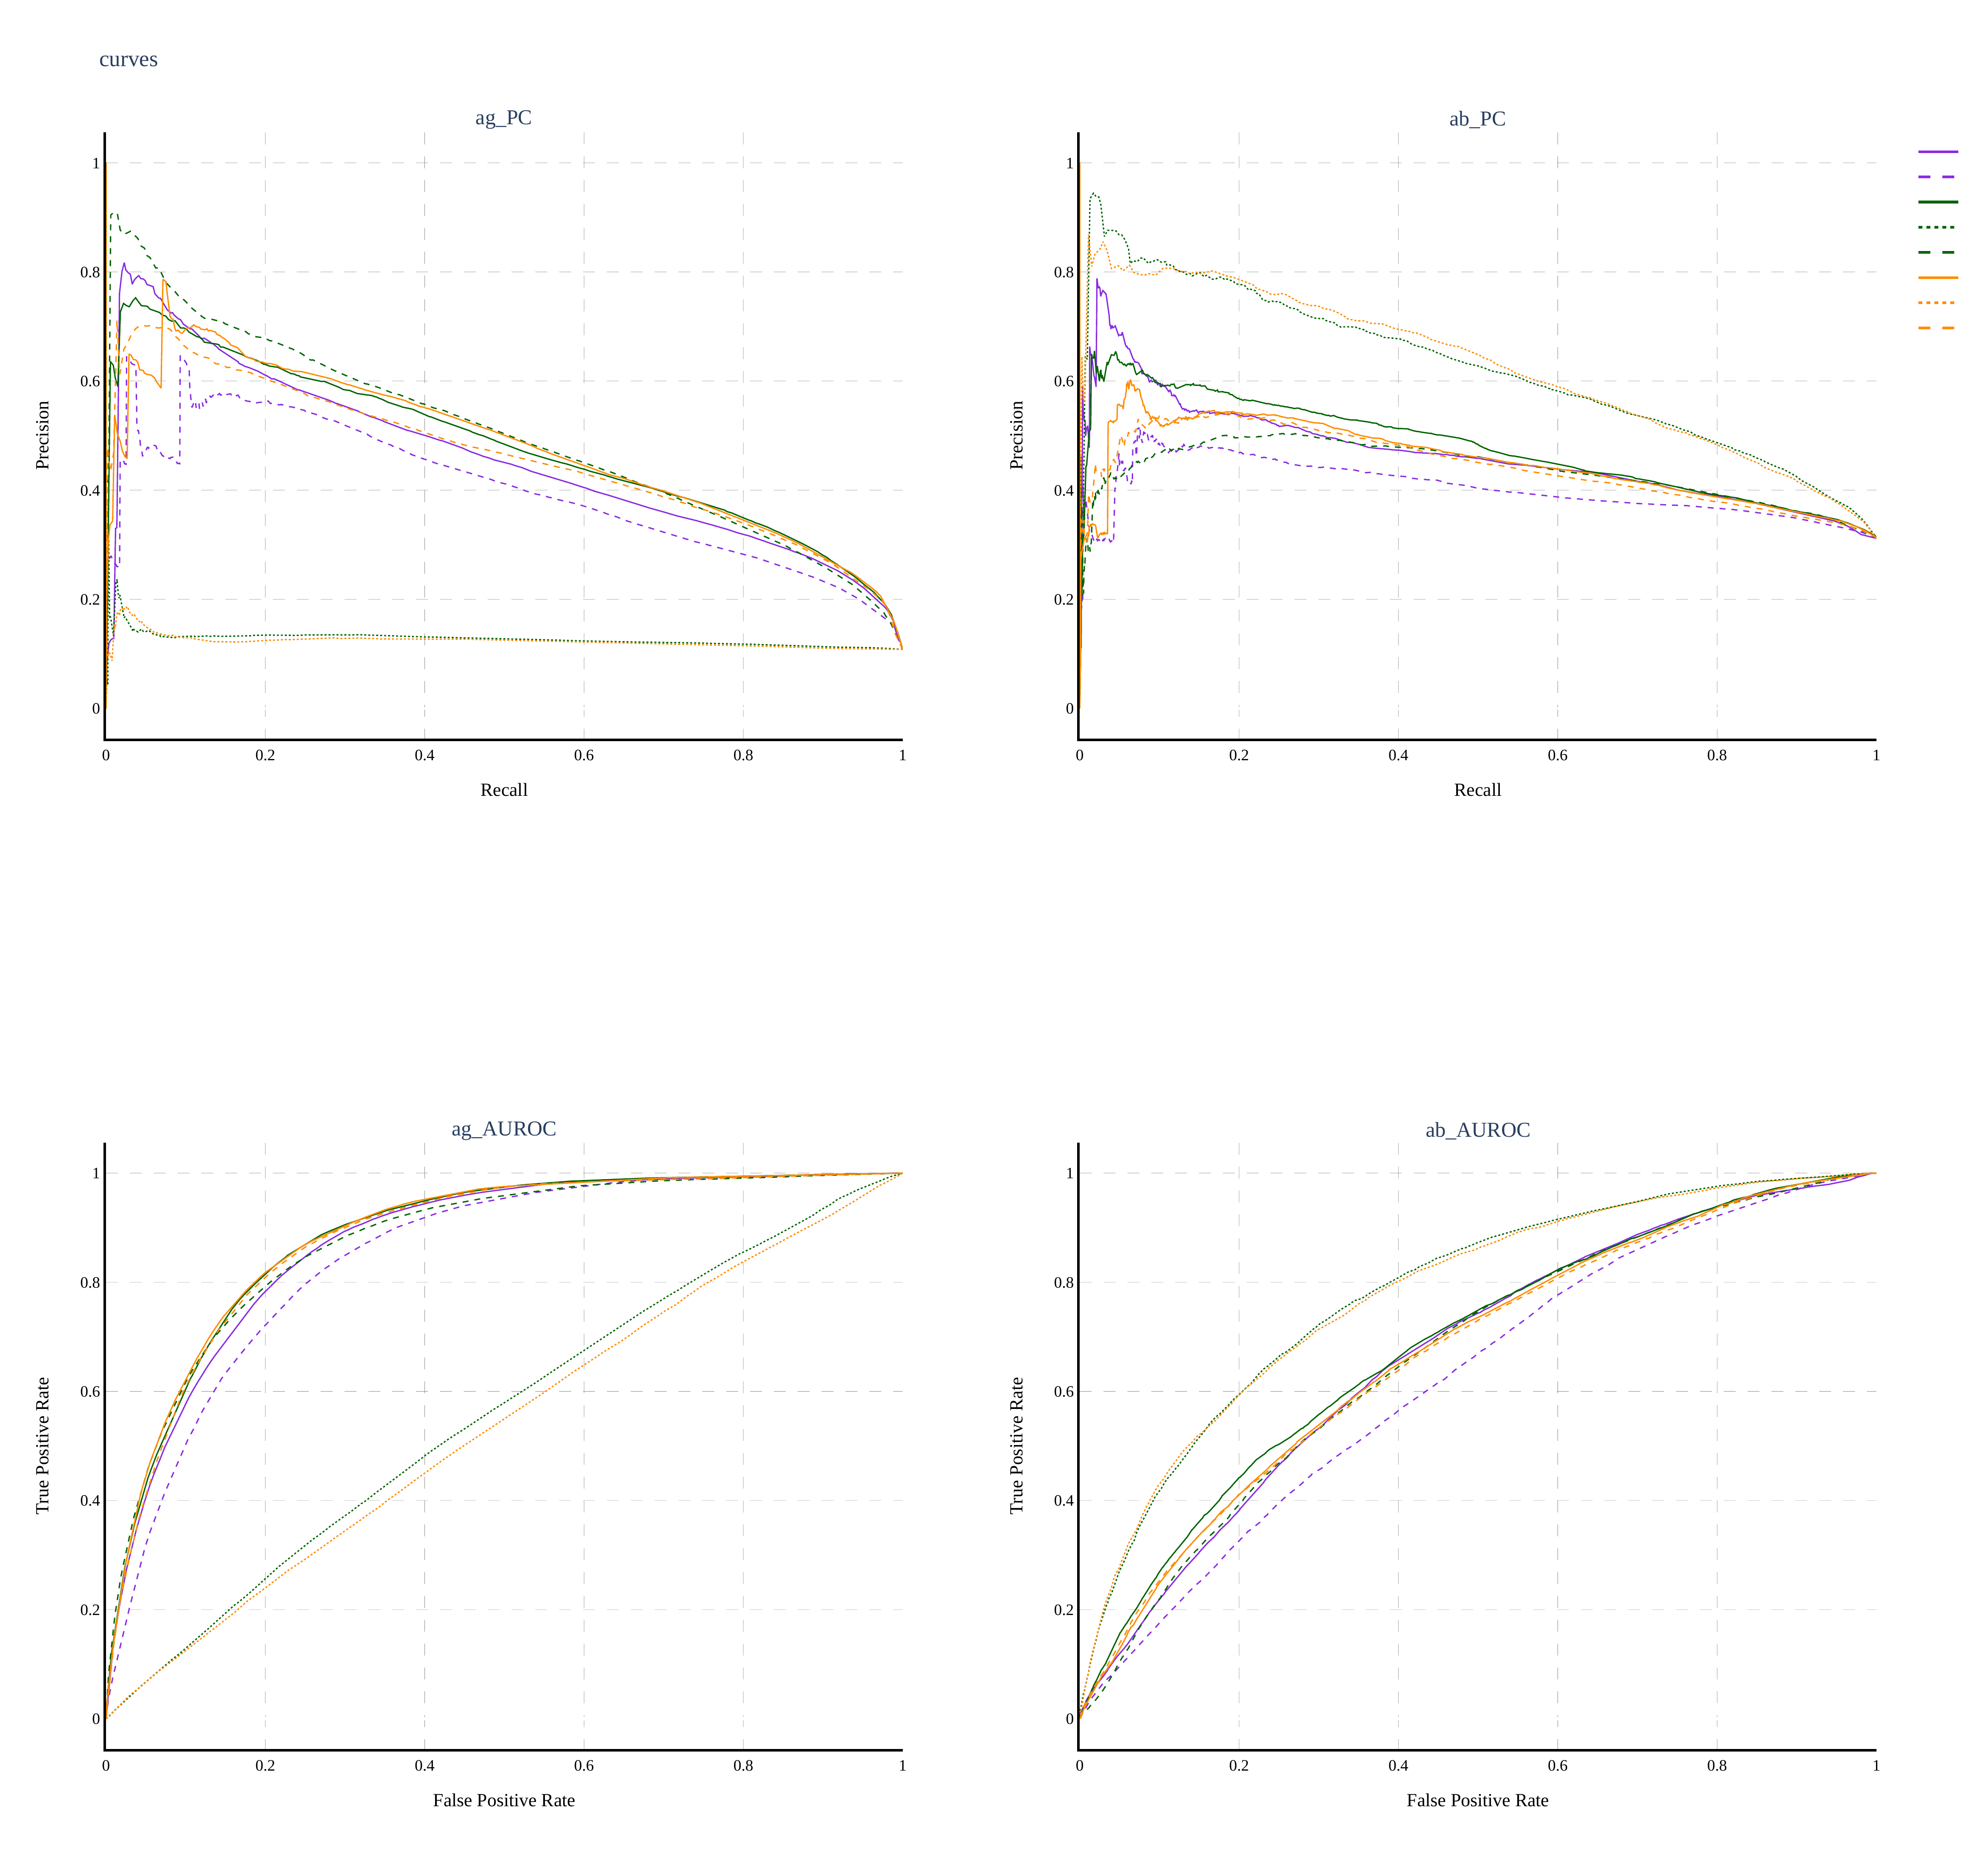}
\put(91,80){\tiny \sc PiNet {\tiny(xyz)}}
\end{overpic}
\caption{\label{fig:surf_curves}}
\end{figure*}
